# Supplementary material for: Language-Guided Audio-Visual Source Separation via Trimodal Consistency
Source: arXiv:2303.16342 source file (2023-09-23)
Supplement: Supplementary file 1 [file 7_supplemental.tex]

% CVPR 2022 Paper Template
% based on the CVPR template provided by Ming-Ming Cheng (https://github.com/MCG-NKU/CVPR_Template)
% modified and extended by Stefan Roth (stefan.roth@NOSPAMtu-darmstadt.de)

\documentclass[10pt,twocolumn,letterpaper]{article}

%%%%%%%%% PAPER TYPE  - PLEASE UPDATE FOR FINAL VERSION
%\usepackage[review]{cvpr}      % To produce the REVIEW version
%\usepackage{cvpr}              % To produce the CAMERA-READY version
\usepackage[pagenumbers]{cvpr} % To force page numbers, e.g. for an arXiv version

% Include other packages here, before hyperref.
\usepackage{graphicx}
\usepackage{amsmath}
\usepackage{amssymb}
\usepackage{booktabs}
\usepackage[pagebackref,breaklinks,colorlinks]{hyperref}
\usepackage{xcolor}         % colors
\usepackage{enumitem}
\usepackage{subfig}
\usepackage{pifont}

%
%

% Support for easy cross-referencing
\usepackage[capitalize]{cleveref}
\crefname{section}{Sec.}{Secs.}
\Crefname{section}{Section}{Sections}
\Crefname{table}{Table}{Tables}
\crefname{table}{Tab.}{Tabs.}

%%%%%%%%% PAPER ID  - PLEASE UPDATE
 % *** Enter the CVPR Paper ID here

\begin{document}

%%%%%%%%% TITLE - PLEASE UPDATE
%
%\title{Sight and Sound of Language: Self-Supervised Natural Language Audio Source Separation in Videos}
\title{Language-Guided Audio-Visual Source Separation via Trimodal Consistency Supplemental Material}

\author{Reuben Tan$^{1}$ \ \ \ \ Arijit Ray$^{1}$ \ \ \ \ Andrea Burns$^{1}$ \ \ \ \ Bryan A. Plummer$^{1}$ \ \ \ \  Justin Salamon $^{2}$ \ \ \ \  \\
Oriol Nieto$^{2}$ \ \ \ \ Bryan Russell$^{2}$ \ \ \ \ Kate Saenko$^{1,3}$ \\
$^{1}$Boston University, $^{2}$Adobe Research, $^{3}$MIT-IBM Watson AI Lab, IBM Research \\
{\tt \small \{rxtan, aburns4, array, bplum, saenko\}@bu.edu}, {\tt \small \{salamon, onieto, brussell\}@adobe.com} \\
} 
\maketitle

\appendix
\input{6_appendix.tex}

%%%%%%%%% REFERENCES
{\small
\bibliographystyle{ieee_fullname}
\bibliography{egbib}
}

\end{document}
